# Supplementary material for: Room temperature ferroic orders in Zr and (Zr, Ni) doped SrTiO$_3$
Source: arXiv:2105.11740 source file (2021-05-25)
Supplement: Supplementary file 1 [file Zr_Ni_Doped_STO_Supp_Information.pdf]

# Supplementary information for
# "Room temperature ferroic orders in Zr and (Zr, Ni) doped $SrTiO_3$"

Shahran Ahmed,[1] A. K. M. Sarwar Hossain Faysal,[1] M. N. I. Khan,[2,*] M. A. Basith,[3,†] Muhammad Shahriar Bashar,[4] H. N. Das,[2] Tarique Hasan,[1] and Imtiaz Ahmed[1,‡]

[1]*Department of Electrical and Electronic Engineering, University of Dhaka, Dhaka-1000, Bangladesh*

[2]*Materials Science Division, Atomic Energy Centre, Dhaka-1000, Bangladesh*

[3]*Nanotechnology Research Laboratory, Department of Physics, Bangladesh University of Engineering and Technology, Dhaka-1000, Bangladesh*

[4]*Institute of Fuel Research and Development, Bangladesh Council of Scientific and Industrial Research, Dhaka-1205, Bangladesh*

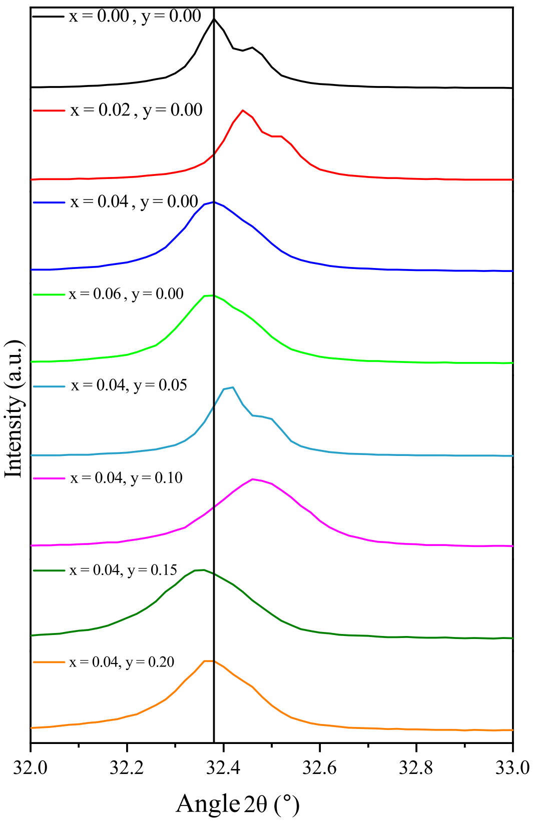


FIG. S1. The evolution of XRD intensity peak of (110) plane of $Sr_{1\text{-}x}Zr_xTi_{1\text{-}y}Ni_yO_3$ for (x, y) = (0.00, 0.00), (0.02, 0.00), (0.04, 0.00), (0.06, 0.00), (0.04, 0.05), (0.04, 0.10), (0.04, 0.15) and (0.04, 0.20).

## XRD PEAK EVOLUTION

The highest intensity peak (110) shifts as Zr and Ni dopants are introduced in the sample, see Fig. S1. These shifts can be attributed to strains induced in the STO cubic structure due to the incorporation of Zr and Ni. Peak shift towards lower diffraction angle usually results from tensile strain due to dopant ions with smaller radii $Zr^{4+}$ ($r_o$ = 0.80 Å) replacing the $Sr^{2+}$ ($r_o$ = 1.26 Å) in A-site; or $Ni^{2+}$ ($r_o$ = 0.69 Å) replacing $Ti^{+4}$ ($r_o$ = 0.74 Å) in B-site. Peak shift towards higher angle results from compressive strain; for example the bigger $Zr^{4+}$ ($r_o$ = 0.80 Å) ion replacing smaller $Ti^{+4}$ ($r_o$ = 0.74 Å). At low Zr concentration such as x=0.02, the XRD peak shifted to higher angle indicating the presence of a compressive strain as some of the $Zr^{4+}$ ions may have substituted the $Ti^{+4}$. But as the Zr concentration was increased to 4% and 6%, the peak moved to lower diffraction angle as more $Zr^{4+}$ ions started

to substitute $Sr^{2+}$. It is evident the peak shift between pure STO and $Sr_{0.96}Ni_{0.04}TiO_3$ is very nominal almost conforming with pure cubic phase. The changes in the full-width-at-half-maximum (FWHM) for (Zr, Ni) co-doped samples indicates slight distortion and disorder due to size differences of substituted dopants and possible interstitial dopants respectively.

## RIETVELD REFINEMENT

| Rietveld refined analysis for Wyckoff position, bond lengths and bond angles | | | | | | | | | | | | | | |
|---|---|---|---|---|---|---|---|---|---|---|---|---|---|---|
| $SrTiO_3$ | | | | | $Sr_{0.96}Zr_{0.04}TiO_3$ | | | | | $Sr_{0.96}Zr_{0.04}Ti_{0.90}Ni_{0.10}O_3$ | | | | |
| atom | site | $x_w$ | $y_w$ | $z_w$ | atom | site | $x_w$ | $y_w$ | $z_w$ | atom | site | $x_w$ | $y_w$ | $z_w$ |
| Sr | 1a | 0 | 0 | 0 | Sr | 1a | 0.0 | 0.0 | 0.0 | Sr | 1a | 0.0 | 0.0 | 0.0 |
| Ti | 1b | 0.5 | 0.5 | 0.5 | Ti | 1b | 0.5 | 0.5 | 0.5 | Ti | 1b | 0.5 | 0.5 | 0.5 |
| O | 3c | 0.0 | 0.5 | 0.5 | O | 3c | 0.0 | 0.5 | 0.5 | O | 3c | 0.0 | 0.5 | 0.5 |
| | | | | | Zr | 1a | 0.0 | 0.0 | 0.0 | Zr | 1a | 0.0 | 0.0 | 0.0 |
| | | | | | | | | | | Ni | 1b | 0.5 | 0.5 | 0.5 |
| Bond length (Å) | | | | | Bond length (Å) | | | | | Bond length (Å) | | | | |
| Ti-O | 1.953 (3) | | | | Ti-O | 1.955 (5) | | | | Ti/Ni-O | 1.957 (6) | | | |
| Sr-O | 2.762 (4) | | | | Sr/Zr-O | 2.762 (4) | | | | Sr/Zr-O | 2.768 (8) | | | |
| Bond angle (°) | | | | | Bond angle (°) | | | | | Bond angle (°) | | | | |
| ⟨Sr-O-Sr⟩ | 90, 180 | | | | ⟨Sr/Zr-O-Sr/Zr⟩ | 90, 180 | | | | ⟨Sr/Zr-O-Sr/Zr⟩ | 90, 180 | | | |
| ⟨Sr-O-Ti⟩ | 90 | | | | ⟨Sr/Zr-O-Ti⟩ | 90 | | | | ⟨Sr/Zr-O-Ti/Ni⟩ | 90 | | | |
| $R_p$ | 5.755 | | | | $R_p$ | 5.334 | | | | $R_p$ | 5.462 | | | |
| $R_{wp}$ | 7.580 | | | | $R_{wp}$ | 7.169 | | | | $R_{wp}$ | 7.32 | | | |
| $R_{exp}$ | 2.023 | | | | $R_{exp}$ | 1.997 | | | | $R_{exp}$ | 1.923 | | | |
| $\chi^2$ | 3.748 | | | | $\chi^2$ | 3.590 | | | | $\chi^2$ | 3.806 | | | |

TABLE S1. Atomic coordinates $x_w$, $y_w$, $z_w$ in Wyckoff notation, bond lengths and bond angles obtained from Rietveld refinement of XRD patterns of $SrTiO_3$, $Sr_{0.96}Zr_{0.04}TiO_3$ and $Sr_{0.96}Zr_{0.04}Ti_{0.90}Ni_{0.10}O_3$.

## EDX PEAK ANALYSIS

To perform chemical species identification of our samples Energy-dispersive X-ray spectroscopy (EDX) spectra for $SrTiO_3$, $Sr_{0.96}Zr_{0.04}TiO_3$ and $Sr_{0.96}Zr_{0.04}Ti_{0.90}Ni_{0.10}O_3$ samples have been obtained as shown in Fig. S2. The atomic weights (%) of chemical species obtained from EDX measurements were compared with corresponding theoretical values for all aforementioned samples, see Table S2.

| EDX Analysis | | | |
|---|---|---|---|
| | Element | EDX Atomic (%) | Theoretical Atomic (%) |
| $SrTiO_3$ | Sr | 15.54 | 20 |
| | Ti | 19.98 | 20 |
| | O | 64.57 | 60 |
| $Sr_{0.96}Zr_{0.04}TiO_3$ | Sr | 16.12 | 19.2 |
| | Ti | 23.96 | 20 |
| | O | 59.25 | 60 |
| | Zr | 0.67 | 0.8 |
| $Sr_{0.96}Zr_{0.04}Ti_{0.90}Ni_{0.10}O_3$ | Sr | 16.58 | 19.2 |
| | Ti | 20.82 | 18 |
| | O | 57.36 | 60 |
| | Zr | 0.54 | 0.8 |
| | Ni | 4.7 | 2 |

TABLE S2. Chemical species identification and concentration analysis using EDX of $SrTiO_3$, $Sr_{0.96}Zr_{0.04}TiO_3$ and $Sr_{0.96}Zr_{0.04}Ti_{0.90}Ni_{0.10}O_3$ samples.

### Raman Peak Assignment

The Raman peaks for $SrTiO_3$, $Sr_{0.96}Zr_{0.04}TiO_3$ and $Sr_{0.96}Zr_{0.04}Ti_{0.9}Ni_{0.1}O_3$ samples were identified with their transverse acoustic (TA), longitudinal acoustic (LA), transverse optical (TO) and longitudinal optical (LO) vibrational phonon modes in Table S3.

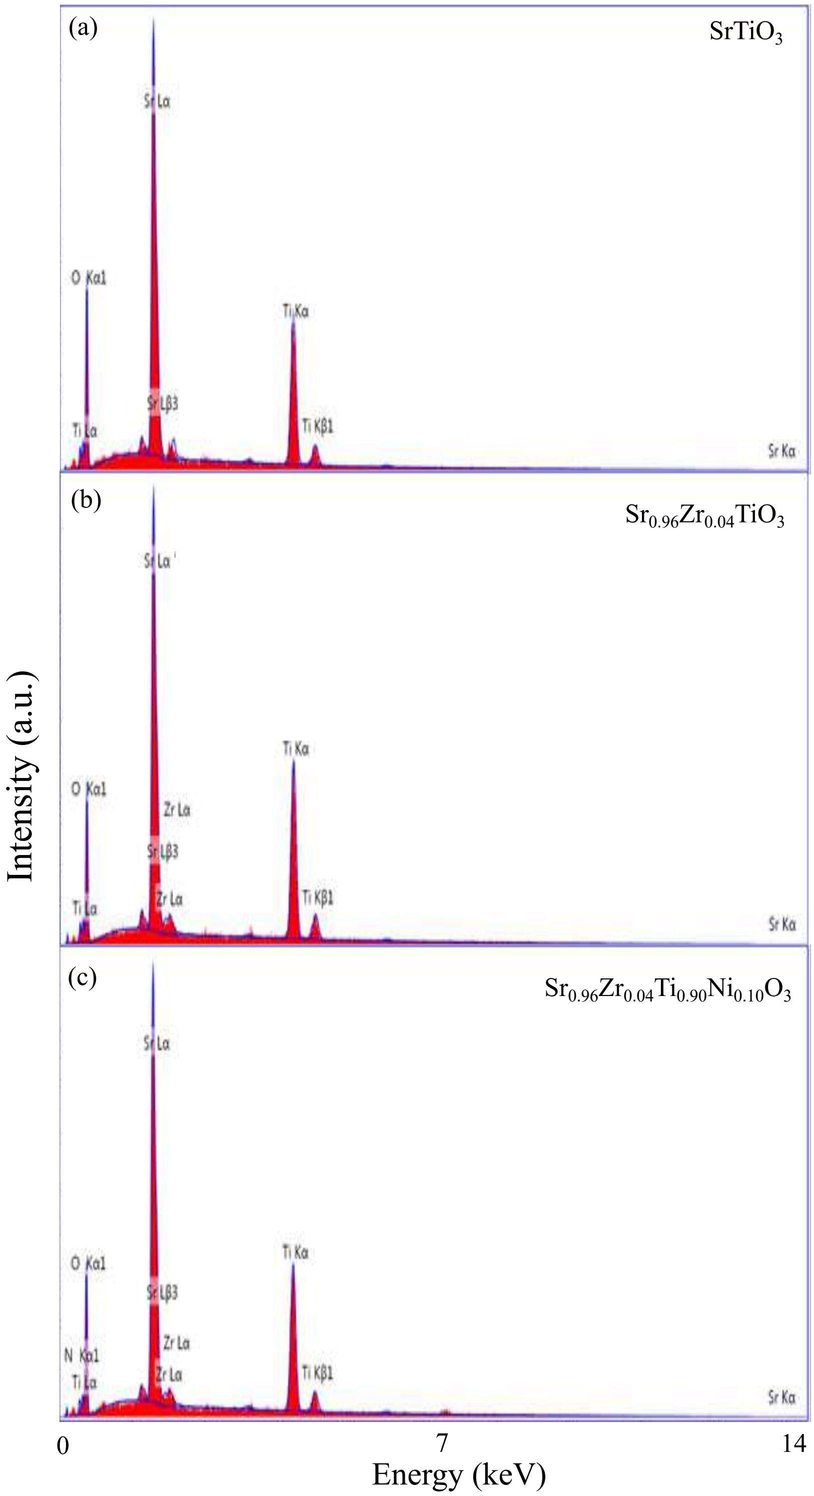


FIG. S2. EDX spectra of (a) $SrTiO_3$, (b) $Sr_{0.96}Zr_{0.04}TiO_3$ and (c) $Sr_{0.96}Zr_{0.04}Ti_{0.90}Ni_{0.10}O_3$.

| Raman Peak Analysis | | | |
|---|---|---|---|
| Peak Assgn. | $SrTiO_3$ ($cm^{-1}$) | $Sr_{0.96}Zr_{0.04}TiO_3$ ($cm^{-1}$) | $Sr_{0.96}Zr_{0.04}Ti_{0.90}Ni_{0.10}O_3$ ($cm^{-1}$) |
| $TO_1$ | 148 | 160 | 145 |
| 2TA | 208 | 201 | 202 |
| $TO_1$+LA | 275 | 285 | 274 |
| $LO_1$+TA, $2TO_2$ | 383 | 377 | 374 |
| $TO_4$ | 547 | - | - |
| $TO_1+TO_4$ | - | 641 | - |
| LA+$LO_3$ | 702 | 701 | 689 |
| $LO_3+TO_2$ | - | - | 762 |
| $LO_4$ | 797 | 800 | - |

TABLE S3. Experimentally observed Raman peak assignments to different phonon vibrational modes of $SrTiO_3$, $Sr_{0.96}Zr_{0.04}TiO_3$ and $Sr_{0.96}Zr_{0.04}Ti_{0.90}Ni_{0.10}O_3$.

**Fourier Transform Infrared Spectroscopy (FTIR)**

The FTIR absorption peaks for $SrTiO_3$, $Sr_{0.96}Zr_{0.04}TiO_3$ and $Sr_{0.96}Zr_{0.04}Ti_{0.90}Ni_{0.10}O_3$ were identified with their chemical bonds vibrations inside the samples in Table S4.

| FTIR Absorption Peak Analysis | | | |
|---|---|---|---|
| Peak Assignment | $SrTiO_3$ ($cm^{-1}$) | $Sr_{0.96}Zr_{0.04}TiO_3$ ($cm^{-1}$) | $Sr_{0.96}Zr_{0.04}Ti_{0.90}Ni_{0.10}O_3$ ($cm^{-1}$) |
| $TiO_2$ | 366 | 366 | 370 |
| $TiO_6$ | 598 | 594 | 536 |
| C-OH | 1462 | 1460 | 1485 |
| -OH | 1653 | 1652 | - |
| -OH | 3465 | 3465 | - |

TABLE S4. Experimentally observed FTIR absorption peak assignment to different chemical bond vibrational modes of $SrTiO_3$, $Sr_{0.96}Zr_{0.04}TiO_3$ and $Sr_{0.96}Zr_{0.04}Ti_{0.90}Ni_{0.10}O_3$.

* ni_khan77@yahoo.com

† mabasith@phy.buet.ac.bd

‡ imtiaz@du.ac.bd
